# Supplementary material for: Anatomizing Deep Learning Inference in Web Browsers
Source: arXiv:2402.05981 source file (2024-07-25)
Supplement: Supplementary file 1 [file appendix.tex]

\onecolumn
\appendix
\section{Appendix: Additional Results}

\input{tex/tab-e2e-native-all}
\input{tex/tab-e2e-tfjs-wasm}

\input{tex/tab-e2e-ort-wasm}
\input{tex/tab-e2e-webgl}

\input{tex/tab-tfjs-warmup-kernel-latency-percentage}
\input{tex/fig-warmup-latency-distribution}

\input{tex/tab-qoe-benchmark}
\begin{table*}[]

    \caption{Smoothness of Web page. The format of each entry, ``/'', ``-D/-I'', and ``M*'' keeps the same as Table~\ref{tab:qoe-merge}.}
    \label{tab:qoe-fps}
    \vspace{-4mm}
    \resizebox{0.95\linewidth}{!}{%
        \begin{tabular}{lrrrrrrrrr}
        \toprule[1.5pt]
                       & \multicolumn{1}{c}{M1} & \multicolumn{1}{c}{M2}         & \multicolumn{1}{c}{M3}         & \multicolumn{1}{c}{M4} & \multicolumn{1}{c}{M5}      & \multicolumn{1}{c}{M6}    & \multicolumn{1}{c}{M7} & \multicolumn{1}{c}{M8} & \multicolumn{1}{c}{M9}    \\ \hline
        TF.js-wasm      & 23.8 (1.83)            & 22.9 (1.79)                    & 22.4 (1.61)                    & 23.9 (1.65)            & /                           & /                         & /                      & /                      & /                         \\
        ORT.js-wasm    & 24.1 (1.79)            & 23.1 (1.49)                    & 24.5 (1.71)                    & 23.8 (1.79)            & 21.7 (1.66)                 & 22.4 (1.66)               & 54.6 (4.07)            & 53.7 (3.71)            & 52.7 (3.51)               \\
        TF.js-WebGL-I   & 11.2 (0.77)            & 11.7 (0.85)                    & 12.9 (1.01)                    & 12.7 (0.82)            & 11.1 (0.84)                 & 11.5 (0.79)               & 26.8 (2.10)            & 27.2 (1.82)            & 23.5 (1.73)               \\
        TF.js-WebGL-D   & 27.2 (1.29)            & 26.4 (1.18)                    & 28.1 (1.51)                    & 28.3 (1.71)            & 27.9 (1.26)                 & 28.1 (1.49)               & 52.4 (2.44)            & 51.5 (3.19)            & 52.0 (2.85)               \\
        ORT.js-WebGL-I & 17.0 (1.11)            & 16.8 (1.11)                    & 17.1 (1.31)                    & /                      & /                           & /                         & /                      & /                      & /                         \\
        ORT.js-WebDL-D & 26.4 (1.39)            & 23.0 (1.08)                    & 24.5 (1.14)                    & /                      & /                           & /                         & /                      & /                      & /                         \\ \bottomrule[1.5pt]
        \end{tabular}%
    }

\end{table*}
\begin{table*}[]

    \caption{Inference accuracy on certain applications. The format of each entry, ``/'', ``-D/-I'', and ``M*'' keeps the same as Table~\ref{tab:qoe-merge}.}
    \label{tab:qoe-dl}
    \vspace{-4mm}
    \resizebox{0.95\linewidth}{!}{%
    \begin{tabular}{lrrrrrr}
    \toprule[1.5pt]
                   & \multicolumn{1}{c}{M1}               & \multicolumn{1}{c}{M2}               & \multicolumn{1}{c}{M3}              & \multicolumn{1}{c}{M4}                & \multicolumn{1}{c}{M5}                & \multicolumn{1}{c}{M6} \\ \hline
    TF.js-Wasm      & 13.7\% (0.53$\times10^{-2}$)         & 13.5\% (0.52$\times10^{-2}$)         & 8.8\% (0.33$\times10^{-2}$)         & 0.78 (2.91$\times10^{-2}$)            & /                                     & /                              \\
    ORT.js-Wasm    & 13.7\% (0.50$\times10^{-2}$)         & 13.6\% (0.52$\times10^{-2}$)         & 8.0\% (0.30$\times10^{-2}$)         & 0.78 (3.10$\times10^{-2}$)            & 0.77 (2.84$\times10^{-2}$)            & 0.79 (3.00$\times10^{-2}$)     \\
    TF.js-WebGL-I   & 8.7\%  (0.33$\times10^{-2}$)         & 8.8\%  (0.32$\times10^{-2}$)         & 3.9\% (0.14$\times10^{-2}$)         & 0.76 (2.86$\times10^{-2}$)            & 0.76 (2.93$\times10^{-2}$)            & 0.78 (2.83$\times10^{-2}$)     \\
    TF.js-WebGL-D   & 14.9\% (0.54$\times10^{-2}$)         & 14.2\% (0.52$\times10^{-2}$)         & 11.1\% (0.44$\times10^{-2}$)        & 0.95 (3.26$\times10^{-2}$)            & 0.94 (3.41$\times10^{-2}$)            & 0.96 (3.59$\times10^{-2}$)     \\
    ORT.js-WebGL-I & 10.5\% (0.39$\times10^{-2}$)         & 11.1\% (0.45$\times10^{-2}$)         & 7.9\% (0.30$\times10^{-2}$)         & /                                     & /                                     & /                              \\
    ORT.js-WebGL-D & 15.1\% (0.57$\times10^{-2}$)         & 15.1\% (0.56$\times10^{-2}$)         & 13.5\% (0.54$\times10^{-2}$)        & /                                     & /                                     & /                              \\ \bottomrule[1.5pt]
    \end{tabular}%
    }

\end{table*}
\twocolumn
